# Supplementary material for: Newton: Gravitating Towards the Physical Limits of Crossbar Acceleration
Source: arXiv:1803.06913 source file (2018-03-10)
Supplement: Supplementary file 1 [file 08-appendix.tex]

\newpage
\vspace{-0.05in}
\section{Appendix}
\label{conclusions}
\vspace{-0.05in}

We have added a new page of content at the start of Section 3 to clearly motivate 
the need for techniques that reduce computation/ADC and why those techniques would 
have little impact in a digital architecture. We have also re-structured the discussion 
of proposals in Section 3 so that (i) Section 3.1 first covers general techniques 
that may apply to any in-situ accelerator, (ii) Section 3.2 then discusses techniques 
to reduce storage/communication costs, and (iii) Section 3.3 puts the many pieces together. 
This re-structuring makes it clear that the proposals have general applicability. 
Most of Section 3.1 can also be understood without deep knowledge of prior work 
(e.g., ISAAC). We also present additional comparison with TPU results to demonstrate 
why the proposed algorithms are best suited for analog over digital designs. 

Reviewers have questioned about the complexity and overhead of the pre/post processing 
of the different optimizations. We highlight that energy cost of modifications to the 
HTree and addition logic for the divide and conquer techniques is less than 1\% in 
comparison to previous analog design. Newton cuts down heavily on usage of analog 
component (ADC+DAC) which contributed to 60\% of power requirement in ISAAC. 
%The storage overheads highlighted in the graphs. 
The buffer reduction technique 
introduces new communication patterns since a layer is distributed across 
several tiles, which gets amortized because adjacent layers get mapped to 
the same tile and hence neurons travel shorter distances.

The applicability of using Newton architecture on large images has been raised before. 
We note that the current Newton architecture can already handle normal (256$\times$256) 
image sizes and easily scales to handle larger (4k resolution) images. Buffer
overhead does increase linearly with image size (only along one
dimension~\cite{shafieenag16}), but as Newton reduces buffer requirement by
4$\times$ the overall buffering overhead is still relatively low. 
%requirement scales with image size and Newton reduces buffer requirement by 4$\times$,

We also quantify the impact of CDAC power in our adaptive ADC scheme based on 
one of the reviews to show that the Adaptive ADC scheme works for most ADC models.

Note that our results focus more on throughput and efficiency and less on
latency. However, a recent work on TPU~\cite{jouppiyoung17} describes a latency
of (7 ms) as a key requirement for many developers. Compared to ISAAC, Newton
tradesoff latency (by 4.5\%) to improve efficiency. However, its overall
latency is still only 6.4 ms even for large networks like VGG-3, which is less than the required threshold. 
%Even though we emphasize throughput, for which the use cases are mobile platforms 
%(self-driving cars, phones) and datacenters, where the chips will be continuously 
%fed with inputs from several cameras or users, we notice in the TPU~\ref{jouppiyoung17} 
%paper that many application developers demand low latency (7 ms). Newton marginally 
%compromises on latency by 4.5\% when compared to ISAAC, due to introduction of 
%additional pre/post processing steps in the pipeline, but is within the tolerance 
%margin (6.4 ms) for large networks like VGG-3. 

Reviewers raised concerns on impact of proposed mapping constraints on general
purpose nature of the accelerator. 
%also questioned about limiting generality of the new optimizations. 
We emphasize that the constraints introduced in the paper do not 
prevent any applications from being mapped to Newton chips, i.e., they do not 
reduce the scope relative to ISAAC. Instead, they reduce area and 
energy for all state-of-the-art large benchmarks.

Both Newton and Eyeriss~\cite{chenemer16} discuss optimizations to reduce
buffering overhead by reusing values.
%In order to highlight our novelty in buffer reduction technique by maximizing 
%neuron input reuse when compared to Eyeriss ~\ref{chenemer16}, we must note 
We note 
that while Eyeriss takes advantage of reuse in the convolution algorithm, 
the reuse in Newton comes from replication of crossbars, which is solely 
due to an analog pipeline. The motivation is the same, but the approach of 
solving it is different: Eyeriss maximizes reuse through a spatial dataflow, 
while Newton uses smart mapping of layers to tiles.

\vspace{0.1in}
\noindent{\bf \large Crossbar Implementations}

Due to some reviews, we discuss in short how crossbars can be designed to withstand
noise effects in analog circuits.

\noindent {\em Process Variation and Noise:}
Since an analog crossbar uses actual conductance of individual cells to perform
computation, it is critical to do writes at maximum precision. We make two 
design choices to improve write precision. First, we equip each cell
with an access transistor (1T1R cell) to precisely control the amount of write
current going through it, eliminating the sneak current
problem~\cite{zangenehjoshi14}. 
Second, we use a closed loop write circuit
with current compliance that does many iterations of program-and-verify
operations~\cite{alibartgao12}. 

In spite of a robust write process, a cell's resistance
will still deviate from its normal value within a tolerable
range. This range will ultimately limit either the 
number of levels in a cell or the number of simultaneously
active rows in a crossbar. For example, if a cell write
can achieve a resistance within $\Delta$r ($\Delta$r is a function of
noise and parasitic), if $l$ is the number of levels in a cell,
and $rrange$ is the max range of resistance of a cell,
then we set the number of active rows to $rrange$/($l$.$\Delta$r)
to ensure there are no corrupted bits at the ADC.

\noindent {\em Crossbar Parasitic:} 
Crossbar accuracy will also get impacted by IR drop along row and columns. A
cell at the far end of the driver will see relatively lower read voltage
compared to a cell closer to the driver. 
This change in voltage is a
function of both wire resistance and the current flowing through wordlines and 
bitlines, which in turn is a function of the data pattern in the array.  This
problem can be addressed by limiting the DAC voltage range and doing data encoding
to compensate for the IR drop~\cite{hustrachan16}. 
Since the matrix being
programmed into a crossbar is known beforehand, during the initialization phase of a
crossbar, it is possible to account for voltage drops and adjust the cell resistance
appropriately.
